# Supplementary material for: Universal behavior of the full particle statistics of one-dimensional Coulomb gases with an arbitrary external potential
Source: arXiv:1803.11269 ancillary file (2018-03-29)
Supplement: Supplementary file 1 [file SI.pdf]

# Supplemental Information: Universal behavior of the full particle statistics of one-dimensional Coulomb gases with an arbitrary external potential


Rafael Díaz Hernández Rojas
*Dipartimento di Fisica, Università di Roma "La Sapienza", P.le A. Moro 5, I-00185 Rome, Italy*

Christopher Sebastian Hidalgo Calva
*Institute of Physics, UNAM, P.O. Box 20-364, 01000 Mexico City, Mexico*

Isaac Pérez Castillo
*Department of Quantum Physics and Photonics, Institute of Physics, UNAM, P.O. Box 20-364, 01000 Mexico City, Mexico and London Mathematical Laboratory, 14 Buckingham Street, London WC2N 6D, United Kingdom*


## MINIMIZING THE HAMILTONIAN

Some of the main features that the equilibrium particles density $\rho_0^*(x)$ acquires in the thermodynamic limit can be computed by finding the optimal configuration in the position of particles, which corresponds to minimizing the Hamiltonian $\mathcal{H}(\mathbf{x})$ (Eq. (2) in the main text). Before proceeding, we highlight the Hamiltonian's invariance upon permutation of particles. This allows us to consider a sorted configuration according to $x_1 < x_2 < \cdots < x_N$, for which we can ignore the absolute value in the one-dimensional Coulomb's potential. Such an ordered Hamiltonian reads

$$\mathcal{H}_o(\mathbf{x}) = N^2 \sum_{i=1}^{N} v(x_i) - N\alpha \sum_{i<j}^{N} (x_j - x_i) \ . \tag{SI-1}$$

We can then find the configurations of particles corresponding to the minimum energy, denoted as $\mathbf{x}^*$, by solving $\frac{\partial \mathcal{H}_o(\mathbf{x})}{\partial x_i}\Big|_{x_i^*} = 0 \ \forall i = 1, ..., N$. We arrive at

$$v'(x_i^*) = \frac{\alpha}{N}(2i - N - 1)\,. \tag{SI-2}$$

The fact that $v''(x) > 0$ for all $x \in [x_-, x_+]$ means that $v'(x)$ is a monotonically increasing function, consistently with the ordered configuration we assumed. Importantly, this also establishes that the inversion needed to solve Eq. (SI-2) for $x_i^*$ can always be carried out in principle. Moreover, the election of powers of $N$ in both terms of the Hamiltonian point out that $\mathcal{O}(x_i) = \mathcal{O}(1)$ but also that we are dealing with a scaled system for which $\mathcal{O}(v(x_i)) = \mathcal{O}(x_i)$. In particular, for the harmonic case , *i.e.* $v(x_i) = \frac{x_i^2}{2}$, the position of the optimal $i$-th particle has the form:

$$x_i^* = \frac{\alpha}{N}\left(2i - N - 1\right) \ . \tag{SI-3}$$

This suggests that the optimal configuration is such that the particles are equidistant and $\rho_0^*(x)$ should be a uniform density. Furthermore, taking the leftmost and rightmost positions, corresponding to $i = 1$ and $i = N$, respectively, we find that the ground state has a natural support $[-\alpha, \alpha]$.

Under the RTM approach, the case of a Wishart–Laguerre ensemble from a $M \times N$ random matrix with $N \leq M$ turns out to be also interesting. In this case the external potential corresponds to $v(x_i) = \frac{1}{2}\left(x_i - a \log x_i\right)$, where $a \equiv \frac{M-N}{N}$. The analysis of the optimal configuration for this case results in:

$$x_i^* = \frac{a}{1 - \frac{2\alpha(2i-N-1)}{N}}. \tag{SI-4}$$

Once again evaluating (SI-4) in the extremal positions yields following inequality:

$$\frac{a}{1 - 2\alpha\left(\frac{1}{N} - 1\right)} < \frac{a}{1 - 2\alpha\left(1 - \frac{1}{N}\right)} \ \xrightarrow[N\to\infty]{} \ \frac{a}{1+2\alpha} < \frac{a}{1-2\alpha}.$$

Whence, in the thermodynamic limit, the support of the equilibrium density for Wishart–Laguerre ensemble is the interval $[\frac{a}{1+2\alpha}, \frac{a}{1-2\alpha}]$. Notice that a necessary condition for these inequalities to hold is that $0 < \alpha < \frac{1}{2}$. This restriction over $\alpha$ allows to confine the gas to a finite support and also guarantees that $V(x)$ dominates over the 1d electrostatic repulsion.

## PDF'S IN THE TYPICAL FLUCTUATIONS REGIME, $F_c(W)$

As it was mentioned for the study of typical fluctuations of the particle $x_i$ around its expect value $\langle x_i\rangle = x_i^*$ , it is constructive to begin with extremal particles, $i = 1$ and $i = N$. Then, for an arbitrary particle $x_K$, with $1 < K < N$, the result will be proportional to the of product of $F_1$ and $F_0$ (Eq. (7) in the main text), corresponding to the CDF of the rightmost and leftmost particles, respectively. Starting from (SI-1), we compute a second order Taylor expansion around $\mathbf{x}^*$:

$$\mathcal{H}_o(\mathbf{x}) \approx \mathcal{H}_o(\mathbf{x}^*) + \frac{N^2}{2}\sum_{i=1}^{N} v''(x_i^*)(x_i - x_i^*)^2 \,. \tag{SI-5}$$

This equation follows as the corresponding Hessian matrix is diagonal. Note, in passing, that a second order expansion is enough, since $x_i - x_i^* \sim \mathcal{O}(1/N)$ and therefore all the remaining terms become negligible in the thermodynamic limit.

We start by considering the probability $F_1(W;N) \equiv \text{Prob}\,[x_1 < x_2 \cdots < x_N < w]$ that $x_N$ has a position smaller than $w$, which we write as a ratio of partition functions $\frac{Z_1(w;N)}{Z_1(\infty;N)}$, where

$$Z_1(w;N) = \int_{-\infty}^{w} dx_N \cdots \int_{-\infty}^{w} dx_2 \int_{-\infty}^{w} dx_1 e^{-\mathcal{H}(\mathbf{x})} \,. \tag{SI-6}$$

We can introduce the ordered Hamiltonian in the expression above and multiply by a factor of $N!$ to compensate the reduction in the integration's volume:

$$\begin{aligned} Z_1(w;N) &= N!\int_{-\infty}^{w} dx_N \cdots \int_{-\infty}^{w} dx_1 e^{-\mathcal{H}(\mathbf{x})} \prod_{i=1}^{N-1}\Theta(x_{i+1}-x_i) \\ &= N!\int_{-\infty}^{w} dx_N \int_{-\infty}^{x_N} dx_{N-1} \cdots \int_{-\infty}^{x_2} dx_1 e^{-\mathcal{H}(\mathbf{x})} \\ &= N!\int_{-\infty}^{w} dx_N \int_{-\infty}^{x_N} dx_{N-1} \cdots \int_{-\infty}^{x_2} dx_1 e^{-\mathcal{H}_o(\mathbf{x})}. \end{aligned} \tag{SI-7}$$

Using the second order approximation of (SI-5) we obtain

$$\begin{aligned} Z_1(w;N) &\approx e^{-\mathcal{H}_o(\mathbf{x}^*)} N! \left[\prod_{i=1}^{N}\int_{-\infty}^{w} dx_i e^{-\frac{N^2}{2}v''(x_i^*)(x_i-x_i^*)^2}\right] \\ &= \frac{e^{-\mathcal{H}_o(\mathbf{x}^*)}N!}{N^N\prod_{i=1}^{N}u_i}\int_{-\infty}^{W} d\epsilon_N e^{-\frac{1}{2}\epsilon_N^2}\left[\prod_{i=1}^{N-1}\int_{-\infty}^{\frac{u_i}{u_{i+1}}\epsilon_{i+1}+\Delta_i^{(+)}} d\epsilon_i e^{-\frac{1}{2}\epsilon_i^2}\right]. \end{aligned} \tag{SI-8}$$

with the definitions $\epsilon_i \equiv N u_i\,(x_i - x_i^*)$, $u_i \equiv \sqrt{v''(x_i^*)}$, $\Delta_i^{(+)} = N u_i(x_{i+1}^* - x_i^*)$ and the scaled random variable $W = N u_N(w - x_N^*)$.

We have thus rewritten $Z_1(w;N)$ as a new partition function where the associated particles have positions $\epsilon_1, \epsilon_2, \ldots, \epsilon_N$ and they are confined by an harmonic potential. Importantly, the ratio $F_1(W;N) = \frac{Z_1(w;N)}{Z_1(\infty;N)}$ corresponds to the CDF of $x_N \leq w$. To overcome the obstacle of a direct evaluation of $Z_1$, we differentiate this CDF (see, for instance Ref. [28]) with respect to $W$ to obtain the probability density function (pdf):

$$\begin{aligned} \frac{dF_1(W;N)}{dW} &= \frac{e^{\frac{-W^2}{2}}}{Z_1(\infty;N)}\int_{-\infty}^{\frac{u_{N-1}}{u_N}W+\Delta_{N-1}^{(+)}} d\epsilon_{N-1}e^{-\frac{1}{2}\epsilon_{N-1}^2}\left[\prod_{i=1}^{N-2}\int_{-\infty}^{\frac{u_i}{u_{i+1}}\epsilon_{i+1}+\Delta_i^{(+)}} d\epsilon_i e^{-\frac{1}{2}\epsilon_i^2}\right] \\ &= \frac{e^{\frac{-W^2}{2}}}{Z_1(\infty;N)} Z_1\left(\frac{u_{N-1}}{u_N}W + \Delta_{N-1}^{(+)}, N-1\right) \\ &= \frac{Z_1(\infty;N-1)}{Z_1(\infty;N)} e^{\frac{-W^2}{2}} F_1\left(\frac{u_{N-1}}{u_N}W + \Delta_{N-1}^{(+)}; N-1\right). \end{aligned} \tag{SI-9}$$

Following Ref. [28], we can argue that the transformed partition function, *i.e.* the one in terms of $\boldsymbol{\epsilon}$, models a system with a short range potential, thus implying that $Z_1(\infty;N) \sim A_1^{-N}$, where $\ln|A_1|$ plays the role of the intensive free

energy. In this way the ratio of the two partition functions in (SI-9) is just $A_1$. As explained in the main text, we expect that in the thermodynamic limit $F$ will be a *universal function* with no dependence on the system's size and, additionally, $\frac{u_{N-1}}{u_N} \to 1$ and $\Delta_{N-1}^{(+)} \to \frac{2\alpha}{u_N}$ when such limit.
The limit of $\Delta_i^{(+)}$ is obtained through the Mean Value Theorem, which states that for a continuous function $f$ in $[a, b]$ and differentiable on $(a, b)$, there exists a $c \in (a, b)$ such that $f'(c) = \frac{f(b)-f(a)}{b-a}$. Applying the theorem to our case with $f = v'$, $a = x_{i-1}^*$, $b = x_i^*$ and using Eq. (SI-2) we have

$$v''(z) = \frac{2\alpha}{N(x_{i+1}^* - x_i^*)}\,, \tag{SI-10}$$

where $z \in (x_i^*, x_{i+1}^*)$. Note that as $N \to \infty$ we can take $z$ as either $x_{i+1}^*$ or $x_i^*$, in particular using the latter we obtain the limit we were looking for $\Delta_i^{(+)} = \frac{2\alpha}{u_i} \approx \frac{2\alpha}{u_{i+1}}$. We can then rewrite (SI-9) as:

$$\frac{dF_1(W)}{dW} = A_1 e^{\frac{-W^2}{2}} F_1\left(W + \frac{2\alpha}{u_+}\right)\,, \tag{SI-11}$$

where we have defined $u_\pm = \sqrt{v''(x\pm)}$. This differential equation can be solved by fixing $A_1$, using the shooting method such that the boundary conditions $F_1(\infty) = 1$ and $F_1(-\infty) = 0$ are fulfilled. Note that these boundary conditions are due to the fact that $F_1$ is a CDF.

Using the same mathematical procedure we can also compute the statisitcs of $x_1$, in which case the probability $\text{Prob}\left[w < x_1 < x_2 \cdots < x_N\right] = \frac{Z_0(w;N)}{Z_0(-\infty;N)}$ has a CDF that can also be expressed as a ratio of partition functions, with

$$\begin{aligned} Z_0(w;N) &= \int_w^\infty dx_1 \cdots \int_w^\infty dx_N e^{-\mathcal{H}(\mathbf{x})} \\ &\approx \frac{e^{-\mathcal{H}_0(\mathbf{x}^*)}N!}{N^N \prod_{i=1}^N u_i} \int_W^\infty d\epsilon_1 e^{-\frac{1}{2}\epsilon_1^2} \left[\prod_{i=2}^N \int_{\frac{u_i}{u_{i-1}}\epsilon_{i-1} - \Delta_i^{(-)}}^\infty d\epsilon_i e^{-\frac{1}{2}\epsilon_i^2}\right]\,, \end{aligned} \tag{SI-12}$$

with $\Delta_i^{(-)} = N u_i \left(x_i^* - x_{i-1}^*\right)$ and $w = N u_1 (x - x_1^*)$. Once again we map the problem into a system with short-range interactions and write the CDF of $x_1$ as $F_0(W) \equiv \frac{Z_0(w;N)}{Z_0(-\infty;N)}$. The corresponding pdf obeys the following differential equation:

$$\frac{dF_0(W)}{dW} = A_0 e^{\frac{-W^2}{2}} F_0\left(W - \frac{2\alpha}{u_-}\right)\,, \tag{SI-13}$$

with the boundary values of $F_0(-\infty) = 1$ and $F_0(\infty) = 0$.

We are now in a position to generalize the previous two results for the $K$-th particle with $1 < K < N$. Let $\text{Prob}\left[x_1 < w, \cdots, x_K < w\right]$ be the CDF of having at least $K = cN$ particles to the left of $w$:

$$\begin{aligned} \text{Prob}\left[x_1 < w, \cdots, x_K < w\right] = \frac{Z_c(w;N)}{Z_c(\infty;N)} &= \frac{1}{Z_c(\infty;N)} \int_{-\infty}^w dx_1 \cdots \int_{-\infty}^w dx_K \int_{-\infty}^\infty dx_{K+1} \cdots \int_{-\infty}^\infty dx_N e^{-\mathcal{H}(\mathbf{x})} \\ &= \frac{N!}{Z_c(\infty;N)} \int_{-\infty}^w dx_K \int_{-\infty}^{x_K} dx_{K-1} \cdots \int_{-\infty}^{x_2} dx_1 \int_{x_K}^\infty dx_{K+1} \cdots \int_{x_{N-1}}^\infty dx_N e^{-\mathcal{H}_o(\mathbf{x})} \\ &\approx \frac{e^{-\mathcal{H}_o(\mathbf{x}^*)}N!}{Z_c(\infty;N)} \int_{-\infty}^w dx_K e^{-\frac{1}{2}N^2 v''(x_K^*)(x_K - x_K^*)^2} \left[\prod_{i=1}^{K-1} \int_{-\infty}^{x_{i+1}} dx_i e^{-\frac{1}{2}N^2 v''(x_i^*)(x_i - x_i^*)^2}\right] \\ &\quad \left[\prod_{i=K+1}^N \int_{x_{i-1}}^\infty dx_i e^{-\frac{1}{2}N^2 v''(x_i^*)(x_i - x_i^*)^2}\right]. \end{aligned} \tag{SI-14}$$

It is straightforward to appreciate that (SI-14) is a combination of (SI-8) and (SI-12), nevertheless we can not put it in terms of $F_1(W; K-1)$ and $F_0(w; N-K)$ yet, since the constants $\Delta_i^{(\pm)}$ correspond to a system of size $N$. We propose the following transformation such that $\Delta_i^{(+)}$ (rep. $\Delta_i^{(-)}$) fits with a system of size $K-1$ (resp. $N-K$). To

find the correct transformation for our case, we derive the general expression for a system of arbitrary size $M$ and a scaled charge magnitude $\alpha'$, so $\Delta_i^{(\pm)}(\alpha, N) \to \Delta_i^{(\pm)}(\alpha', M)$. From Eq. (SI-2),

$$v'(x_i^*(\alpha, N)) - v'(x_i^*(\alpha', M)) = 2i\left(\frac{\alpha}{N} - \frac{\alpha'}{M}\right) - (\alpha - \alpha') - \left(\frac{\alpha}{N} - \frac{\alpha'}{M}\right) = \alpha\left(\frac{M}{N} - 1\right). \tag{SI-15}$$

Where in the last equality we set $\alpha' = M/N$ so the difference of $v(x_i^*)$'s for any subsystem will be a constant. We now introduce an auxiliary transformed variable $\xi_i$ determined according to $Nu_i(\alpha, N)x_i = Mu_i(\alpha', M)\xi_i$. Hence, each term of the sum in the exponential's argument in Eq. (SI-14) can be reexpressed as

$$N^2 u_i^2(\alpha, N)\left[x_i - x_i^*(\alpha, N)\right]^2 = M^2 u_i^2(\alpha', M)\left[\xi_i - \frac{Nu_i(\alpha, N)}{Mu_i(\alpha', M)} x_i^*(\alpha, N)\right]^2 \equiv M^2 u_i^2(\alpha', M)\left[\xi_i - \xi_i^*\right]^2. \tag{SI-16}$$

We now let $M = K$ and define, just as before, new integration variables, $\epsilon_i^{(+)} \equiv Ku_i(\alpha', K)\left[\xi_i - \xi_i^*\right]$. When neglecting factors of the form $\frac{u_i}{u_{i\pm1}}$, since they converge to unit for large enough systems, the upper integration limit becomes $y_{i+1}^{(+)} \equiv \epsilon_{i+1}^{(+)} + \Delta_i^{(+)}$ with $\Delta_i^{(+)}(\alpha', K) = Ku_i(\alpha', K)\left(\xi_{i+1}^* - \xi_i^*\right)$. Similarly, for a system of size $N - K$, which models the particles to the right of $x_K$, we use a transformed (and shifted) variable $Nu_{i+k}(\alpha, N)x_{i+K} = Mu_i(\alpha', M)\zeta_i$:

$$N^2 u_{i+K}^2(\alpha, N)\left[x_{i+K} - x_{i+K}^*(\alpha, N)\right]^2 = M^2 u_i^2(\alpha', M)\left[\zeta_i - \frac{Nu_{i+K}(\alpha, N)}{Mu_i(\alpha', M)} x_{i+K}^*(\alpha, N)\right]^2 \equiv M^2 u_i^2(\alpha', M)\left[\zeta_i - \zeta_i^*\right]^2. \tag{SI-17}$$

We then let $M = N - K$ and define $\epsilon_i^{(-)} \equiv (N-K)u_i(\alpha', N-K)\left[\zeta_i - \zeta_i^*\right]$ with the lower integration limit as $y_{i-1}^{(-)} \equiv \epsilon_{i-1}^{(-)} - \Delta_i^{(-)}$. Finally, being $\epsilon_K \equiv Ku_K(\alpha, K)(x_K - x_K^*)$ and $W \equiv Nu_K(\alpha, N)(w - x_K^*(\alpha, N))$, it is easy to conclude that $y_K^{(+)} = \epsilon_K + \Delta_{K-1}^{(+)}$ and $y_0^{(+)} = \epsilon_K - \Delta_1^{(-)}$ and transform (SI-14) into:

$$\begin{aligned} \text{Prob}\left[x_1 < w, \cdots, x_K < w\right] &\approx A_c \int_{-\infty}^{W} \mathrm{d}\epsilon_K\, e^{-\frac{1}{2}\epsilon_K^2}\left[\prod_{i=1}^{K-1}\int_{-\infty}^{y_{i+1}^{(+)}} \mathrm{d}\epsilon_i\, e^{-\frac{1}{2}\epsilon_i^2}\right]\left[\prod_{i=1}^{N-K}\int_{y_{i-1}^{(-)}}^{\infty} \mathrm{d}\epsilon_i\, e^{-\frac{1}{2}\epsilon_i^2}\right] \\ &= A_c \int_{-\infty}^{W} \mathrm{d}\epsilon_K\, e^{-\frac{1}{2}\epsilon_K^2} F_1\left(y_K^{(+)}; K-1\right) F_0\left(y_0^{(-)}; N-K\right) \equiv F_c(W). \end{aligned} \tag{SI-18}$$

where $A_K$ is related to the normalization condition:

$$A_c^{-1} = \int_{-\infty}^{\infty} \mathrm{d}\epsilon_K\, e^{-\frac{1}{2}\epsilon_K^2} F_1\left(y_K^{(+)}\right) F_0\left(y_0^{(-)}\right). \tag{SI-19}$$

Differentiating (SI-18) we finally obtain a relation for the pdf:

$$\frac{dF_c(W)}{dW} = A_c e^{-\frac{1}{2}W^2} F_1\left(W + \Delta_{K-1}^{(+)}\right) F_0\left(W - \Delta_1^{(+)}\right). \tag{SI-20}$$

As a last step, we also notice that for large enough systems and subsystems, *i.e.* the ratios $c = K/N$ and $N - K/N$ remain finite in the thermodynamic limit, we can approximate $\Delta_i^{(\pm)}(\alpha', M) \approx \Delta_i^{(\pm)}(\alpha, N)$ for $M = K$ or $M = N - K$ and any $i = 1, \ldots, N$. Applying the mean value theorem as above, it is straightforward to show that

$$\Delta_i^{(+)}(\alpha', K) \approx Nu_i(\alpha, N)\left[\frac{2\alpha}{Nu_i^2(\alpha, N)}\right] = \frac{2\alpha}{u_i(\alpha, N)} \tag{SI-21a}$$

$$\Delta_i^{(-)}(\alpha', N-K) \approx Nu_{K+i}\left[\frac{2\alpha}{Nu_{K+i}^2(\alpha, N)}\right] = \frac{2\alpha}{u_{K+i}(\alpha, N)} \tag{SI-21b}$$

Whence we can conclude that $\Delta_K^{(+)}(\alpha', K) = \Delta_0^{(-)}(\alpha', N-K) \approx \Delta_1^{(-)}(\alpha', N-K)$, this last approximation being exact in the infinite subsystem limit. Defining $2\alpha/u_c$ as the value of these delay and lag terms in such a limit we recover Eq. (7) of the main text.

### Asymptotic behavior of $F_c'(W)$

We can follow the procedure described in Ref. [28] to derive an expression for the asymptotic of $F_1'(W)$, as $W \to \infty$. To do so, we begin from the forward differential equation Eq. SI-11 and note that as $W \to \infty$, $F_1(W) \to 1$, since it is a CDF, whence we clearly obtain that the asymptotic behavior is simply $\exp\left(-\frac{W^2}{2}\right)$. The other limit, *i.e.* $W \to -\infty$ is analyzed proposing an ansatz of the form $F_1(W) \asymp \exp(-\kappa_1 |W|^\gamma)$ and then plugging it into Eq. (SI-11) to determine $\kappa_1$ and $\gamma$ by equating powers of $|W|$ in the exponentials' arguments. When doing so, the resulting expression to leading order becomes

$$F_1'(W) \asymp \exp(-\kappa_1 |W|^\gamma) \asymp \exp\left(-\frac{W^2}{2} - \kappa_1 \left|W + \frac{2\alpha}{u_+}\right|^\gamma\right) \asymp \exp\left(-\frac{W^2}{2} - \kappa_1 |W|^\gamma + \frac{2\alpha\kappa_1\gamma}{u_+}|W|^{\gamma-1}\right).$$

By equating powers of $|W|$ so that they cancel identically we clearly arrive at $\gamma = 3$ and $\kappa_1 = \frac{u_+}{12\alpha}$. An entirely analogous analysis can be done for the asymptotic behavior of the pdf of $x_{\min}$, proposing $F_0(W) \asymp \exp(-\kappa_0 |W|^\gamma)$, where once again it is found that $\gamma = 3$ and now $\kappa_0 = \frac{u_-}{12\alpha}$.

Next, we apply the same technique to study $F_c'(W)$ for large values of $|W|$ and for $0 < c < 1$. We begin from Eq. (7) of the main text, using the same ansatz proposed above for $F_0(W)$ (resp. $F_1(W)$), but recalling that, as derived above, this CDF should be obtain for a delay (resp. forward) term equal to $\frac{2\alpha}{u_c}$. This means our anzats are now $F_0(W) \asymp \exp\left(-\frac{u_c}{12\alpha}W^3\right)$ and $F_1(W) \to 1$ as $W \to \infty$. It is a remarkable result that when we plug these expression in Eq. (10), the quadratic term cancels and we end up with an exponential with a cubic dependence, *i.e.* a non-Gaussian behavior, namely, $F_c'(W) \asymp \exp\left(-\frac{u_c}{12\alpha}W^3\right)$. When considering the case $W \to -\infty$ we arrive at exactly the same conclusion. So in summary, the asymptotic behavior of $F_c'$ is given by

$$F_0'(W) \asymp \begin{cases} \exp\left(-\frac{W^2}{2}\right), & W \to -\infty \\ \exp\left(-\frac{u_-}{12\alpha}W^3\right), & W \to \infty\,, \end{cases} \tag{SI-22a}$$

$$F_1'(W) \asymp \begin{cases} \exp\left(-\frac{u_+}{12\alpha}|W|^3\right), & W \to -\infty \\ \exp\left(-\frac{W^2}{2}\right), & W \to \infty\,, \end{cases} \tag{SI-22b}$$

$$F_c'(W) \asymp \exp\left(-\frac{u_c}{12\alpha}|W|^3\right), \quad W \to \pm\infty, \quad 0 < c < 1\,. \tag{SI-22c}$$

Therefore we recover Eqs. (8) and (9) from the main text. We show below that this asymptotic behavior matches exactly the third order expansion of the rate function.

## DERIVING THE PARTICLES DENSITY, $\rho_0^*(x)$ AND $\rho^*(x)$

Here we focus on the derivations which guide us to get an analytic expression for the particles density function $\rho(x)$. Using a path integral representation together with the Saddle-Point method we will solve the probability that the have a a fraction $c = K/N$ of particles to the left of $w$, which is equivalent that the Kth particle would be equal to $w$. We introduce $\rho\left(x|\{x_i\}_{i=1}^N\right) = \frac{1}{N}\sum_{i=1}^N \delta(x_i - \lambda)$ to rewrite (Eq. (10) in the main text) as:

$$\varrho(c,w) = \frac{1}{\Omega_0}\int \mathrm{d}\mathbf{x}\, e^{\mathcal{H}[\rho(x|\{x_i\}_{i=1}^N)]}\delta\left[c - \int dx \Theta(w-x)\rho(x|\{x_i\}_{i=1}^N)\right]. \tag{SI-23}$$

Here, the expression

$$\mathcal{H}[\rho(x|\{x_i\}_{i=1}^N)] = N^3 \int dx\, v(x)\rho\left(x|\{x_i\}_{i=1}^N\right) - \frac{\alpha}{2}N^3 \int dx dx'\, |x - x'| \rho\left(x|\{x_i\}_{i=1}^N\right)\rho\left(x'|\{x_i\}_{i=1}^N\right) \tag{SI-24}$$

corresponds to a Hamiltonian from one-dimensional CG with and arbitrary external potential (Eq. (2) in the main text). Introducing a functional Dirac delta in its Fourier representation we turn the simple integral into a double path integral:

$$\varrho(c,w) = \frac{1}{\Omega_0}\int D[\rho,\widehat{\rho}]e^{\Gamma[\rho,\widehat{\rho}]}\delta\left[c - \int dx\, \rho(x)\Theta(w-x)\right], \tag{SI-25}$$

with the functional $\Gamma[\rho,\widehat{\rho}] = \mathcal{H}[\rho] - iN\int dx\widehat{\rho}(x)\rho(x) - N\ln\left(\int dx e^{-i\widehat{\rho}(x)}\right)$. We can now approximate the path integral over $\hat{\rho}$ by the saddle-point method, obtaining the following saddle-point equation:

$$\rho(x) = \frac{e^{-i\widehat{\rho}_0(x)}}{\int dx\, e^{-i\widehat{\rho}_0(x)}}. \tag{SI-26}$$

This implies that $\rho(x)$ is normalized. Secondly, after taking the logarithm of this result, multiplying by $\rho(x)$, and integrating with respect to $x$, we find that the entropic term, $\int dx\rho(x)\ln(\rho(x)) = -i\int dx\widehat{\rho}_0(x)\rho(x) - \ln\left(\int dx e^{-i\widehat{\rho}_0(x)}\right)$, scales as $\mathcal{O}(N)$. Thus, we can neglect it, and after imposing the normalization condition via a Dirac delta we obtain:

$$\varrho(c,w) \asymp \frac{1}{\Omega_0}\int D[\rho]e^{\Gamma[\rho,\widehat{\rho}_0]}\delta\left[c - \int dx\,\rho(x)\Theta(w-x)\right]\delta\left[1 - \int dx\,\rho(x)\right] = \frac{1}{\Omega_0}\int D[\rho,\mu,\nu]e^{S[\rho,\mu,\nu]}. \tag{SI-27}$$

where the action $S[\rho,\mu,\nu]$ is given by Eq. (11) in the main text, once we have taken the Fourier representation of the Dirac deltas, using $\nu$ and $\mu$ as integration variables. We apply the saddle-point method once again, this time over $\rho(x)$, $\mu$, and $\nu$, to obtain the asymptotic behaviour:

$$\varrho(c,w) \approx \frac{1}{\Omega_0}e^{S[\rho^*,\mu^*,\nu^*]}\,, \tag{SI-28}$$

where $\rho^*(x)$, $\mu^\star$, and $\nu^\star$ obey the following saddle-point equations:

$$\frac{\delta S[\rho^*,\mu^*,\nu^*]}{\delta\rho(x)} = v(x) - \alpha\int dx'|x-x'|\rho^*(x') + \mu^* + \nu^*\,\Theta(w-x) = 0\,, \tag{SI-29}$$

$$\frac{\partial S[\rho^*,\mu^*,\nu^*]}{\partial\mu} = 1 - \int dx\,\rho^*(x) = 0\,, \tag{SI-30}$$

$$\frac{\partial S[\rho^*,\mu^*,\nu^*]}{\partial\nu} = c - \int dx\,\Theta(w-x)\rho^*(x) = 0\,. \tag{SI-31}$$

The saddle-point equations for $\rho_0^*(x)$ is similarly obtained by extremizing $S[\rho,\mu_0]$ yielding $v(x)-\alpha\int dx'|x-x'|\rho_0^*(x') + \mu_0^\star = 0$. The solution to this equation is found by recalling that $\frac{d^2|x-x'|}{dx^2} = 2\delta(x-x')$, so that by differentiating twice this last saddle-point equation we get:

$$\rho_0^*(x) = \frac{v''(x)}{2\alpha}\mathbb{I}[x_- \le x \le x_+]\,. \tag{SI-32}$$

We have added an indicator function to write down explicitly its support, so that we are left to determining the values of $x_\pm$. Plugging the solution (SI-32) back into its saddle-point equation yields:

$$2v(x) - \int_{x_-}^{x_+} dx'|x-x'|v''(x) + 2\mu_0^\star = (v'(x_-)+v'(x_+))x - (\chi(x_-)+\chi(x_+)-2\mu_0^\star) = 0\,, \tag{SI-33}$$

where $\chi(x) = xv'(x) - v(x)$. Since Eq. to (SI-33) must be obeyed $\forall x \in [x_-, x_+]$, this implies that:

$$v'(x_-) + v'(x_+) = 0\,, \tag{SI-34}$$

$$\chi(x_-) + \chi(x_+) - 2\mu_0^* = 0\,. \tag{SI-35}$$

In addition, the normalization conditions results into:

$$\int dx\,\rho_0^*(x) = \frac{v'(x_+) - v(x_-)}{2\alpha} = 1. \tag{SI-36}$$

Therefore, from Eqs. (SI-34) and (SI-36) we get that $v'(x_\pm) = \pm\alpha$.

To obtain the solution $\rho^*(x)$ obeying the saddle-point equations (SI-29), (SI-30), and (SI-31), we first notice that, due to the inter-particle potential, we expect that excess particles will accrue on the wall and that a gap will open between $w$ and some value $x_0$. With a modest amount of foresight, we propose an expression of $\rho^*(x)$ to be a weighted

sum of $\rho_0^*(x)$ with a non-compact support plus a Dirac delta placed at the wall:

$$\rho^*(x) = \begin{cases} \frac{v''(x)}{2\alpha}\mathbb{I}_{[x_- \le x < x_0]} + \gamma(c,w)\delta(w-x), & x_+ < w \\ \\ \frac{v''(x)}{2\alpha}\mathbb{I}_{[x_- \le x < w]} + \frac{v''(x)}{2\alpha}\mathbb{I}_{[x_0 < x \le x_+]} + \gamma(c,w)\delta(w-x), & c > c^*(w) \\ \\ \frac{v''(x)}{2\alpha}\mathbb{I}_{[x_- < x \le x_0]} + \frac{v''(x)}{2\alpha}\mathbb{I}_{[w \le x < x_+]} + \gamma(c,w)\delta(w-x), & c < c^*(w) \\ \\ \frac{v''(x)}{2\alpha}\mathbb{I}_{[x_0 \le x < x_+]} + \gamma(c,w)\delta(w-x), & w < x_- \end{cases} . \tag{SI-37}$$

Here, the function $\gamma(c, w)$ is the weight that measures the fraction of particles accumulated on the wall. In the ansatz (SI-37) we have also introduced the quantity $c^*(w)$ given by:

$$c^*(w) = \int_{x_-}^{w} dx \rho_0^*(x) = \frac{v'(w) - v'(x_-)}{2\alpha}\,, \tag{SI-38}$$

which corresponds to the natural fraction of particles $c$ such that the wall is ineffective. As the position of the wall is free, we can naturally extend this definition outside the natural support of $\rho_0^*(x)$ by simply writing:

$$c^*(w) = \begin{cases} 1, & x_+ < w \\ \frac{v'(w)-v'(x_-)}{2\alpha}, & x_- \le w \le x_+ \\ 0, & w < x_- \end{cases} . \tag{SI-39}$$

We are left with the task of determining the parameters $x_0$ and $\gamma(c, w)$ appearing in the expression (SI-37). To do so, we need to evaluate this ansatz on the saddle-point equations (SI-29), (SI-30), and (SI-31). Indeed, let us, for instance, consider the case of $c > c^*(w)$ in (SI-37) and substitute it into the saddle-point equation (SI-31). This yields $\gamma(c, w) = c - c^*(w)$. Furthermore, plugging this ansatz into the saddle-point equation (SI-29), and recalling that the corresponding result must be valid for all values of $x$, we obtain either that

$$v'(x_-) + v'(w) + v'(x_+) - v'(x_0) + 2\alpha\gamma(c, w) = 0\,, \tag{SI-40}$$
$$\chi(x_-) + \chi(w) + \chi(x_+) - \chi(x_0) + 2\alpha w\gamma(c, w) - 2\mu^\star - 2\nu^\star = 0\,, \tag{SI-41}$$

for $x \le w$, or

$$v'(x_-) - v'(w) + v'(x_+) + v'(x_0) - 2\alpha\gamma(c, w) = 0\,, \tag{SI-42}$$
$$\chi(x_-) - \chi(w) + \chi(x_+) + \chi(x_0) - 2\alpha w\gamma(c, w) - 2\mu^\star = 0\,, \tag{SI-43}$$

for $w < x$. The set of equations (SI-40), (SI-41), (SI-42), (SI-43), together with the result $\gamma(c, w) = c - c^*(w)$, and the normalization condition, provides a closed system of equations for the parameters $x_0$ and $\gamma(x, w)$ appearing in (SI-37), and the Lagrange multipliers $\mu^*$ and $\nu^*$.

This derivation can be naturally extended to the remainder cases appearing in the ansatz (SI-37). All in all, the weight becomes $\gamma = |c - c^*(w)|$, with $v'(x_0) = \alpha(2c - 1)$. Moreover, the Lagrange multipliers $\nu^*$m $\mu^*$ are written as follows:

$$\nu^* = \begin{cases} \alpha w(1-2c) + v(w) + \chi(x_0), & & x_+ < w \\ \\ 2\alpha\gamma w + \chi(w) - \chi(x_0), & c > c^*(w), & x_- \le w \le x_+ \\ \\ 2\alpha\gamma w + \chi(x_0) - \chi(w), & c < c^*(w), & x_- \le w \le x_+ \\ \\ \alpha w(2c-1) - v(w), & & w < x_- \end{cases} , \tag{SI-44}$$

and

$$\mu^* = \begin{cases} \frac{1}{2}\left[\chi(x_-) - \chi(x_0) + 2\alpha c w - 2v(w)\right], & x_+ < w \\ \\ \frac{1}{2}\left[\chi(x_-) + \chi(x_+) - \nu^*\right], & x_- \le w \le x_+ \\ \\ \frac{1}{2}\left[\chi(x_+) - \chi(x_0) - 2\alpha c w\right], & w < x_- \end{cases} . \tag{SI-45}$$

We next particularise our results to the two paradigmatic external potentials of RMT corresponding to the Gaussian and the Wishart-Laguerre ensembles, *i.e*:

$$\mathcal{H}_{\mathrm{GE}}(\mathbf{x}) = \frac{1}{2}N^2\sum_{i=1}^{N} x^2 - \alpha N \sum_{i<j}^{N} |x_i - x_j|\,, \tag{SI-46}$$

$$\mathcal{H}_{\mathrm{WE}}(\mathbf{x}) = \frac{1}{2}N^2\sum_{i=1}^{N} (x - a\ln(x)) - \alpha N \sum_{i<j}^{N} |x_i - x_j|\,. \tag{SI-47}$$

For the first case, the density $\rho^\star(x)$ reads:

$$\rho^*_{\mathrm{GE}}(x) = \begin{cases} \frac{1}{2\alpha}\mathbb{I}_{[\alpha,x_0]} + (1-c)\delta(w-x), & \alpha < w. \\ \\ \frac{1}{2\alpha}\mathbb{I}_{[-\alpha,w]} + \frac{1}{2\alpha}\mathbb{I}_{[x_0,\alpha]} + |c - c^*(x)|\delta(w-x), & c > c^*(x). \\ \\ \frac{1}{2\alpha}\mathbb{I}_{[-\alpha,\lambda_0]} + \frac{1}{2\alpha}\mathbb{I}_{[w,\alpha]} + |c^*(x) - c|\delta(x-\lambda), & c < c^*(x). \\ \\ \frac{1}{2\alpha}\mathbb{I}_{[x_0,\alpha]} + c\delta(w-x), & w < -\alpha. \end{cases} , \tag{SI-48}$$

with $x_0 = 2\alpha\left(1 - \frac{1}{2}\right)$, $c^*(w) = \frac{1}{2}\left(1 + \frac{w}{\alpha}\right)$ for $w \in [-\alpha, \alpha]$. Moreover $\rho^*_0(x) = \frac{1}{2\alpha}\mathbb{I}_{[-\alpha,\alpha]}$. For the second case, we have instead that:

$$\rho^*_{\mathrm{WE}}(x) = \begin{cases} \frac{a}{4\alpha x^2}\mathbb{I}_{\left[\frac{a}{1+2\alpha},x_0\right]} + (1-c)\delta(x-\lambda), & \frac{a}{1-2\alpha} < w. \\ \\ \frac{a}{4\alpha x^2}\mathbb{I}_{\left[\frac{a}{1+2\alpha},w\right]} + \frac{a}{4\alpha x^2}\mathbb{I}_{\left[x_0,\frac{a}{1-2\alpha}\right]} + |c - c^*(x)|\delta(x-\lambda), & c > c*(x). \\ \\ \frac{a}{4\alpha x^2}\mathbb{I}_{\left[\frac{a}{1+2\alpha},x_0\right]} + \frac{a}{4\alpha x^2}\mathbb{I}_{\left[w,\frac{a}{1-2\alpha}\right]} + |c - c^*(x)|\delta(x-\lambda), & c < c*(x). \\ \\ \frac{a}{4\alpha x^2}\mathbb{I}_{\left[x_0,\frac{a}{1-2\alpha}\right]} + c\delta(x-\lambda), & w < \frac{a}{1+2\alpha}. \end{cases} . \tag{SI-49}$$

Here $x_0 = \frac{a}{1-2\alpha(2c-1)}$, $c^*(w) = \left[\frac{1}{4\alpha}\left(1 - \frac{a}{w}\right) + \frac{1}{2}\right]$ with $w \in \left[\frac{a}{1+2\alpha}, \frac{a}{1-2\alpha}\right]$, and $\rho^*_0(x) = \frac{a}{4\alpha x^2}\mathbb{I}_{\left[\frac{a}{1+2\alpha},\frac{a}{1-2\alpha}\right]}$.

## DERIVATION OF THE RATE FUNCTIONS

To study the behavior of the atypical fluctuation we compute the rate function as the difference between the Hamiltonian constricted to the SIN and this one when the gas is in its the equilibrium state, *i.e.* $\psi(c, w) = S[\rho^*, \mu^*, \nu^*] - S_0[\rho^*_0, \mu^*_0]$. Notice that the action, at the saddle point can be written in terms of one integral only by noticing that if we multiply (SI-29) by $\rho^*(x)$ and integrate with respect to $x$ we get:

$$\alpha \int dx \int dx' |x - x'| \rho^*(x)\rho^*(x') = \int dx v(x)\rho^*(x) + \mu^* + c\nu^*\,. \tag{SI-50}$$

This allows us to replace the double integral in the action to become:

$$S[\rho^*, \mu^*, \nu^*] = \frac{1}{2}\left[\int dx v(x)\rho^*(x) - \mu^* - c\nu^*\right]\,. \tag{SI-51}$$

Similarly, for the unconstrained case we have that

$$S_0[\rho_0^*, \mu_0^*] = \frac{1}{2}\left[\int dx v(x)\rho_0^*(x) - \mu_0^*\right] . \tag{SI-52}$$

The last step consists in substituting the solution (SI-37) for $\rho^*(x)$ and $\rho_0^*(x)$ into the two aforementioned expressions. As the solution for the constrained density is given in a piece-wise manner, we need to discuss the cases separately. When $w \in [x_-, x_+]$ the action becomes:

$$S[\rho^*, \mu^*, \nu^*] = \frac{1}{2}\left[\left(\int_{x_-}^{a} dx \frac{v''(x)v(x)}{2\alpha} + \int_{b}^{x_+} dx \frac{v''(x)v(x)}{2\alpha} + |c - c^*(x)|v(w)\right) - \mu^* - c\nu^*\right] . \tag{SI-53}$$

For $c > c^*(w)$ (resp. $c < c^*(w)$) we must take $a = w$ and $b = x_0$ (resp. $a = x_0$ and $b = w$). When deriving the rate function $\psi(c, w)$, it is convenient to split the limits of the integral appearing in (SI-52) into two parts, from $[x_-, x_0]$ and then $[x_0, x_+]$. This eventually yields the following expression for the rate function:

$$\psi(c, w) = \frac{1}{2}\left[|c - c^*(x)|v(w) - \int_{a}^{b} dx \frac{v''(x)v(x)}{2\alpha} + \mu_0^* - \mu^* - c\nu^*\right] . \tag{SI-54}$$

The case of $x_+ < w$ (resp. $w < x_-$) in the ansatz (SI-37) yields the precisely the same expression of the rate function but with the choices $b = x_+$, $a = x_0$ and $|c - c^*(w)| = (1 - c)$ (resp. $b = x_0$ , $a = x_-$ and $|c - c^*(w)| = c$).

We can particularise for the Gaussian and Wishart-Laguerre esnembles. For the first case the rate function becomes:

$$\psi_{\mathrm{GE}}(c, w) = \begin{cases} \frac{(1-c)\left[\alpha^2(1-c)^2+3(w-\alpha c)^2\right]}{6}, & \alpha < w \\ -\frac{(\alpha(1-2c)+w)^3}{12\alpha}, & c > c^*(w) \\ \frac{(\alpha(1-2c)+w)^3}{12\alpha}, & c < c^*(w) \\ \frac{c\left[\alpha^2c^2+3(w+\alpha(1-c))^2\right]}{6}, & w < -\alpha \end{cases} , \tag{SI-55}$$

while for the Wishart-Laguerre ensemble we have instead:

$$\psi_{\mathrm{WE}}(c, w) = \begin{cases} \frac{4\alpha(1-c)\left[a\ln\left|\frac{a}{w\eta}\right|+w(1+2\alpha c)\right]-a(1-2\alpha)\ln\left|\frac{\eta}{1-2\alpha}\right|}{8\alpha}, & \frac{a}{1-2\alpha} < w \\ \frac{a^2-w^2\eta^2+2aw\eta\ln\left|\frac{w\eta}{a}\right|}{16w\alpha}, & c > c^*(w) \\ -\frac{a^2-w^2\eta^2+2aw\eta\ln\left|\frac{w\eta}{a}\right|}{16w\alpha}, & c < c^*(w) \\ \frac{4\alpha c\left[a\ln\left|\frac{a}{w\eta}\right|+w(1+2\alpha(1-c))\right]+a(1+2\alpha)\ln\left|\frac{\eta}{1+2\alpha}\right|}{8\alpha}, & x < \frac{a}{1+2\alpha} \end{cases} , \tag{SI-56}$$

with the definition $\eta = (1 - 2\alpha(2c - 1))$.

As shown in [16,19], the rate function, as a function of $w$ with $c$ fixed describes the large deviations for the $K$-th particle, while as a function of $c$ with $w$ fixed, describes the large deviation of the fraction of particles to the left of $w$. It was also proven in [16,19] that it is possible to recover both left and right rate functions of extremal particles in as unified way. Indeed, the limits:

$$\phi_M^{(-)}(w) = \lim_{c\to 1^-} \psi(c, w), \quad w \le x_+ , \tag{SI-57}$$

$$\phi_M^{(+)}(w) = \lim_{c\to 1^-} \frac{\psi(c, w)}{1 - c}, \quad w \ge x_+ , \tag{SI-58}$$

yield the rate functions $\phi_M^{(-)}(w)$ and $\phi_M^{(+)}(w)$ which describe the atypical fluctuation when $x_{\max} \equiv x_+$ is pushed to the left or to the right of $w$, respectively. The factor $1-c$ is responsible for the change of scaling from $\mathcal{O}(N^3)$ to $\mathcal{O}(N^2)$ between the push and pull mechanisms describing the large deviations of the rightmost particle [16,19]. Similarly, we can define $\phi_m^{(+)}(w)$ and $\phi_m^{(-)}(w)$ as the limits

$$\phi_m^{(-)}(w) = \lim_{c\to 0^+} \frac{\psi(c,w)}{c}, \quad w \le x_-\,, \tag{SI-59}$$

$$\phi_m^{(+)}(w) = \lim_{c\to 0^+} \psi(c,w), \quad w \ge x_-\,, \tag{SI-60}$$

$$\tag{SI-61}$$

which yield, similarly as before, the rate functions $\phi_m^{(-)}(w)$ and $\phi_m^{(+)}(w)$ the atypical fluctuations of the leftmost particle $x_{\min} \equiv x_-$.

Applying these general result to the the harmonic potential, the atypical fluctuations for rightmost particle read:

$$\phi_{\mathrm{GE,M}}^{(-)}(w) = \begin{cases} \frac{(\alpha-w)^3}{12\alpha}, & w \in [-\alpha,\alpha] \\ \frac{w^2}{2} + \frac{\alpha^2}{6}, & w < -\alpha \end{cases}, \tag{SI-62}$$

and

$$\phi_{\mathrm{GE,M}}^{(+)}(w) = \frac{(w-\alpha)^2}{2} \quad w \ge \alpha\,, \tag{SI-63}$$

consistent with the findings in [28]. Due to the symmetry of the harmonic potential the rate function of the leftmost particle is attained by $w \to -w$ in the previous expressions. For the Wishart external potential the rate functions for the rightmost particle are:

$$\phi_{\mathrm{WE,M}}^{(-)}(w) = \begin{cases} \frac{a^2 - w^2(1-2\alpha)^2 + 2\alpha w(1-2\alpha)\ln\left|\frac{w(1-2\alpha)}{a}\right|}{16\alpha w}, & w \in \left[\frac{a}{1+2\alpha}, \frac{a}{1-2\alpha}\right] \\ \frac{4\alpha\left(w + a\ln\left|\frac{a}{w}\right|\right) + a\left(\ln\left|\frac{1-2\alpha}{1+2\alpha}\right| - 2\alpha\ln\left|1-4\alpha^2\right|\right)}{8\alpha}, & w < \frac{a}{1+2\alpha} \end{cases}, \tag{SI-64}$$

and

$$\phi_{\mathrm{WE,M}}^{(+)}(w) = \frac{w(1-2\alpha) + a\left(\ln\left|\frac{a}{w(1-2\alpha)}\right| - 1\right)}{2}, \quad w > \frac{a}{1-2\alpha}\,. \tag{SI-65}$$

For the leftmost particle, the rate functions read:

$$\phi_{\mathrm{WE,m}}^{(+)}(w) = \begin{cases} -\frac{a^2 - w^2(1+2\alpha)^2 + 2\alpha w(1+2\alpha)\ln\left|\frac{w(1+2\alpha)}{a}\right|}{16\alpha x}, & w \in \left[\frac{a}{1+2\alpha}, \frac{a}{1-2\alpha}\right] \\ \frac{4\alpha\left(w + a\ln\left|\frac{a}{w}\right|\right) + a\left(\ln\left|\frac{1-2\alpha}{1+2\alpha}\right| - 2\alpha\ln|1-4\alpha^2|\right)}{8\alpha}, & w > \frac{a}{1-2\alpha} \end{cases}, \tag{SI-66}$$

and

$$\phi_{\mathrm{WE,m}}^{(-)}(w) = \frac{w(1+2\alpha) + a\left(\ln\left|\frac{a}{w(1+2\alpha)}\right| - 1\right)}{2}, \quad w < \frac{a}{1+2\alpha}\,. \tag{SI-67}$$

## DISCONTINUOUS THIRD DERIVATIVE OF $\psi(c,w)$

We begin by investigating the small deviations of the particles positions around their optimal position, $w^*$ or, likewise, small deviations of the of the fraction of particles to the left of the wall from $c^*$. In the former case, $w^* = w^*(c)$ is the optimal position of the wall that would constrain a fraction $c$ of particles to its left. Its value can be found by inverting Eq. (SI-39) and letting $c \in [0,1]$ to vary freely. When doing so, we find that $w^*(c) = x_0(c)$, and we will therefore use the two variables interchangeably. The probability of such small deviations will be described by the first non-vanishing term of the Taylor series of $\psi$ around $(c^*, w^*)$. Note that this point is precisely the global minimum of the rate function, at which it becomes 0. Hence, the first term of the Taylor expansion is to be considered are the

second partial derivatives. Using the several relations defined above for the parameters involved in the expression of $\psi$ and assuming that $c > c^*$ (or equivalently, $w < w^*$), by direct differentiation we find that

$$\frac{\partial^2\psi(c,w)}{\partial w^2} = (c - c^*(w))v''(w), \tag{SI-68a}$$

$$\frac{\partial^2\psi(c,w)}{\partial c^2} - 2\alpha(w - w^*(c)), \tag{SI-68b}$$

$$\frac{\partial^2\psi(c,w)}{\partial c\partial w} = -2\alpha(c - c^*(w))\,. \tag{SI-68c}$$

These equations identically vanish once the LHS are evaluated at $c = c^*$, $w = w^*$. This is a remarkable result, for it signals a departure from the Gaussian behavior reported in the 2d case. With this in mind, we consider the next relevant terms for the series expansion, related to the third derivatives:

$$\frac{\partial^3\psi(c,w)}{\partial w^3} = (c - c^*(w))v'''(w) - \frac{v''(w)^2}{2\alpha}, \tag{SI-69a}$$

$$\frac{\partial^3\psi(c,w)}{\partial c^3} = \frac{4\alpha^2}{v''(x_0(c))}\,, \tag{SI-69b}$$

and similar expressions for the crossed derivatives. These expressions are in general different from zero even at $(c^*, w^*)$. The case $c < c^*$ (or equivalently $w > w^*$) just changes a global sign to these equations, hence indicating that the third derivatives of the rate function are in general, discontinuous. When Eq. (SI-69a) is used to approximate the probability

$$\Pr(x_i = w) \sim \exp\big(-N^3\psi(c^*, w)\big) \asymp \exp\left(-\frac{N^3}{3!}\frac{\partial^3\psi(c^*,w^*)}{\partial w^3}|w - w^*|^3\right) \tag{SI-70}$$

we recover exactly Eq. (SI-22c), thus proving that the rate function matches smoothly with the pdf once we are in the large deviations regime.

Although this result seems to suggest that the applicability of the rate function could be extended to the typical fluctuations regime, we now give numerical evidence that this is not the case. The reason for this rather unexpected limitation is that the last expression only agrees with Eq. (SI-22c) once the asymptotic behavior of the latter has taken over. However, before large fluctuations are dominant, there should be, in fact, a quadratic term in the exponential's argument to be able to approximate the form of $F_c'(W)$ around its mode. This is shown in Fig. SI-1, where we compare the exact expression of $F_c'(W)$ (blue curve), with the pdf computed using the closed form of the rate function (red curve) and the approximation of Eq. (SI-70) (green, dashed curve). The orange dashed curve is a numerical fit to $\log F_c'(W)$ considering a polynomial with non-vanishing quadratic and cubic terms, while the cyan line is a fit to the same data, but using a fit where only $|w - w*|^3$ is considered. This thus provides another example of a system where the non-analyticity and non-strict convexity of the rate function near its minimum impedes its usage for a description of the typical fluctuations regime.

For simplicity we have restricted our analysis to the region $x_- \leq w \leq_+$, but an analogous treatment can be done for the other values of $w$ outside the natural support of the particle density.

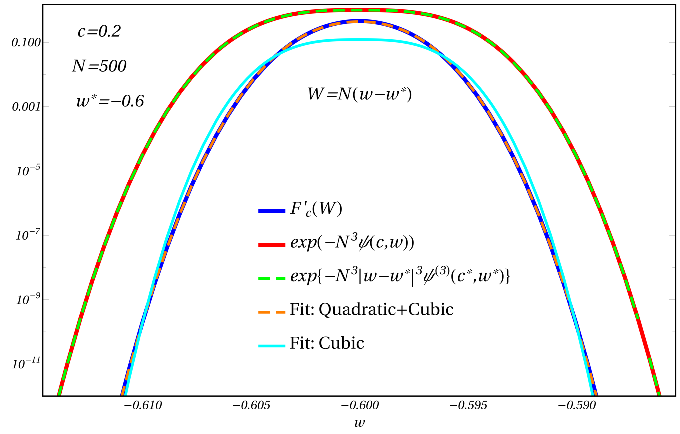


FIG. SI-1. Comparison of the exact PDF given by Eq. (7) in main text, of the fluctuations around $w^*$ in the harmonic potential (blue solid curve) with the distribution obtain using the rate function around its minimum (red solid curve) for the harmonic potential. The green dash line shows that the third order expansion of Eq. (SI-70) matches perfectly the exact behavior for small fluctuations. Finally, we also analyzed the form of the exact PDF by fitting $\log_{10} F_c'(W)$ a polynomial containing quadratic and cubic terms (orange dashed line) and only a cubic term (cyan curve).
